# Supplementary material for: Correction of Density-Functional-Theory based polynomial interatomic potentials to reproduce experimental melting properties
Source: arXiv:2110.02660 ancillary file (2021-10-06)
Supplement: Supplementary file 1 [file supplemental_material.pdf]

# Supplemental Material: Correction of Density-Functional-Theory based polynomial interatomic potentials to reproduce experimental melting properties

Bernd Bauerhenne[1], Martin E. Garcia[1]

October 6, 2021

[1] Theoretical Physics and Center for Interdisciplinary Nanostructure Science and Technology (CINSaT), Heinrich-Plett-Straße 40, 34132 Kassel, Germany

Correspondence to: bauerhenne@uni-kassel.de

# Contents

1 **Analytical form of the interatomic potential** **S-1**

2 **Electronic temperature dependent interatomic potential coefficients for the melting temperature corrected silicon potential** **S-2**

3 **Fortran implementation of the interatomic potential** **S-6**

# 1 Analytical form of the interatomic potential

To facilitate the understanding of this section, we now repeat the equations (2) - (6) of the research paper. We construct $\Phi(T_\mathrm{e})$ as the sum of the following local interaction terms:

$$\begin{aligned}\Phi \;=\; & \sum_{i} \Phi_0(T_\mathrm{e}) + \sum_{\substack{i<j \\ r_{ij}<r_2^{(\mathrm{c})}}} \Phi_2(T_\mathrm{e}, r_{ij}) + \sum_{\substack{i\,j\,k \\ r_{ij}, r_{ik} < r_3^{(\mathrm{c})}}}{}' \, \Phi_3(T_\mathrm{e}, r_{ij}, r_{ik}, \theta_{ijk}) \\ & + \sum_i \Phi_\rho\left(T_\mathrm{e}, \rho_i^{(2)}, \rho_i^{(3)}, \ldots, \rho_i^{\left(N_\rho^{(r)}\right)}\right). \qquad \text{(S1)}\end{aligned}$$

Here $r_{ij}$ denotes the distance between atoms $i$ and $j$, $\theta_{ijk}$ is the angle between $\mathbf{r}_{ij}$ and $\mathbf{r}_{ik}$, the prime indicates that all summation indices are distinct, and $\rho_i^{(2)}$, $\rho_i^{(3)}, \ldots$ are different measures for the atomic density surrounding atom $i$ (see below).
We expand the terms $\Phi_2$, $\Phi_3$, $\Phi_\rho$ and also $\rho_i^{(2)}, \rho_i^{(3)}, \ldots$ into *polynomials*, which can, in principle, reproduce any physically reasonable function. To achieve high numerical stability, the polynomials must be functions of variables lying in the interval $[-1, 1]$. Hence, we use $\cos(\theta)$, where $\theta$ is a bond angle, and $1-r/r^{(\mathrm{c})}$, being $r$ an interatomic distance, as variables for the polynomials. The powers of the latter start from degree two to let $\Phi(T_\mathrm{e})$ and its first derivatives continuously decreasing to zero as distances reach the cutoff radii. Thus, $\Phi_2$, $\Phi_3$ are constructed as

$$\Phi_2 = \sum_{q=2}^{N_2^{(r)}} c_2^{(q)} \left(1 - \frac{r_{ij}}{r_2^{(\mathrm{c})}}\right)^q, \tag{S2}$$

$$\Phi_3 = \sum_{q_1=2}^{N_3^{(r)}} \sum_{q_2=q_1}^{N_3^{(r)}} \sum_{q_3=0}^{N_3^{(\theta)}} c_3^{(q_1\, q_2\, q_3)} \left(1 - \frac{r_{ij}}{r_3^{(\mathrm{c})}}\right)^{q_1} \left(1 - \frac{r_{ik}}{r_3^{(\mathrm{c})}}\right)^{q_2} \Big(\cos(\theta_{ijk})\Big)^{q_3}, \tag{S3}$$

and, for $q_1 = 2, 3, \ldots, N_\rho^{(r)}$, the measures for the atomic density surrounding atom $i$ are constructed as

$$\rho_i^{(q_1)} = \sum_{\substack{j \neq i \\ r_{ij} < r_\rho^{(\mathrm{c})}}} \left(1 - \frac{r_{ij}}{r_\rho^{(\mathrm{c})}}\right)^{q_1}. \tag{S4}$$

By definition, $\rho_i^{(q_1)} \in [0, \infty)$, and if all of them are zero, then $\Phi_\rho$ should be also zero. Hence, to construct $\Phi_\rho$, we use powers of $\rho/(1+\rho)$, starting from degree one, for expanding the atomic density $\rho$, since $\rho/(1+\rho)$ is zero for $\rho = 0$ and converges to one for $\rho \to \infty$:

$$\Phi_\rho = \sum_{q_1=2}^{N_\rho^{(r)}} \sum_{q_2=1}^{N_\rho^{(\rho)}} c_\rho^{(q_1\, q_2)} \left(\frac{\rho_i^{(q_1)}}{1+\rho_i^{(q_1)}}\right)^{q_2}. \tag{S5}$$

# 2 Electronic temperature dependent interatomic potential coefficients for the melting temperature corrected silicon potential

The interatomic potential $\Phi(T_\mathrm{e})$ has the polynomial degrees

$$N_2^{(r)} = 10, \qquad N_3^{(r)} = 3, \qquad N_3^{(\theta)} = 3 \qquad N_\rho^{(\rho)} = 2, \qquad N_\rho^{(r)} = 2 \tag{S6}$$

and needs therefore in total 23 coefficients. The two-body term $\Phi_2$ has 9, the three-body term $\Phi_3$ has 12, and the embedding function $\Phi_\rho$ has 2 coefficients. Furthermore, the cutoff radii

$$r_2^{(\mathrm{c})} = 6.3 \text{ Å}, \qquad r_3^{(\mathrm{c})} = 4.2 \text{ Å}, \qquad r_\rho^{(\mathrm{c})} = 4.8 \text{ Å} \tag{S7}$$

are constant and do not depend on the electronic temperature $T_\mathrm{e}$. The $T_\mathrm{e}$-dependence of the coefficients was fitted to a polynomial of degree 5. Hence, any coefficient $c$ of the interatomic potential depends on $T_\mathrm{e}$ as

$$c = \sum_{k=0}^{5} a^{(k)} \left( \frac{T_\mathrm{e}}{31577\,\mathrm{K}} \right)^k . \tag{S8}$$

In order to describe the parametrization of the term $\Phi_0(T_\mathrm{e})$, let us consider an isolated atom. It contains discrete energy levels of the electrons. The electronic occupation of these energy levels is given by a Fermi distribution with $T_\mathrm{e}$. Since there are big gaps between the discrete energy levels in the atom, the internal energy $U_0$ and the entropy $S_0$ of the atom do not change with increasing $T_\mathrm{e}$ at low $T_\mathrm{e}$'s. Consequently, the Helmholtz free energy

$$\Phi_0(T_\mathrm{e}) = U_0 - T_\mathrm{e}\, S_0 \tag{S9}$$

of the isolated atom is a linear function of $T_\mathrm{e}$ at low $T_\mathrm{e}$'s. Starting from $\sim$ 4500 K, the internal energy $U_0$ and the entropy $S_0$ start depending on $T_\mathrm{e}$. Above this temperature, the Helmholtz free energy $\Phi_0(T_\mathrm{e})$ behaves in a non-linear fashion. Hence, the Helmholtz free energy $\Phi_0(T_\mathrm{e})$ of an isolated atom was fitted to a polynomial of degree 1 at $T_\mathrm{e} \leq 4500$ K and to a polynomial of degree 13 at $T_\mathrm{e} > 4500$ K:

$$\Phi_0(T_\mathrm{e}) = \begin{cases} a_0^{(0)} + a_0^{(1)} \left(\frac{T_\mathrm{e} - 4500\,\mathrm{K}}{31577\,\mathrm{K}}\right), & T_\mathrm{e} \leq 4500\,\mathrm{K}; \\ a_0^{(0)} + a_0^{(1)} \left(\frac{T_\mathrm{e} - 4500\,\mathrm{K}}{31577\,\mathrm{K}}\right) + \sum\limits_{k=4}^{13} a_0^{(k)} \left(\frac{T_\mathrm{e} - 4500\,\mathrm{K}}{31577\,\mathrm{K}}\right)^k, & T_\mathrm{e} > 4500\,\mathrm{K}. \end{cases} \tag{S10}$$

By construction of $\Phi_0(T_\mathrm{e})$, its first, second, and third derivative are continuous functions of $T_\mathrm{e}$.
The parametrization of the interatomic potential is tabulated in Tabs. S1 - S4. The unit of the coefficients is eV and the unit of $T_\mathrm{e}$ is K. The fitted range of the polynomial expansion yields 316 K $\leq T_\mathrm{e} \leq$ 31577 K.

**Table S1:** Parametrization of $c_2^{(q)} = \sum\limits_{k=0}^{5} a_2^{(k\,q)} \left(\frac{T_\mathrm{e}}{31577\,\mathrm{K}}\right)^k$ for the two-body term $\Phi_2$, see Eq. (S2).

| $k$ | $q$ | $a_2^{(k\,q)}$ | $k$ | $q$ | $a_2^{(k\,q)}$ | $k$ | $q$ | $a_2^{(k\,q)}$ |
|---|---|---|---|---|---|---|---|---|
| 0 | 2 | -0.652029301662623 | 0 | 3 | -19.0589296869611 | 0 | 4 | 546.769257376815 |
| 1 | 2 | 9.26314534875668 | 1 | 3 | -400.089680112155 | 1 | 4 | 6319.96355713893 |
| 2 | 2 | -50.0186051618631 | 2 | 3 | 2167.05447438595 | 2 | 4 | -35385.6550126843 |
| 3 | 2 | 115.557349548295 | 3 | 3 | -4520.34437699249 | 3 | 4 | 71794.8635849514 |
| 4 | 2 | -114.529669723874 | 4 | 3 | 4095.42902709553 | 4 | 4 | -62858.4678911266 |
| 5 | 2 | 40.7054174379305 | 5 | 3 | -1352.35365149216 | 5 | 4 | 20099.4017864489 |

*continuation on next page ...*

*continuation from last page*

| $k$ | $q$ | $a_2^{(k\,q)}$ | $k$ | $q$ | $a_2^{(k\,q)}$ | $k$ | $q$ | $a_2^{(k\,q)}$ |
|---|---|---|---|---|---|---|---|---|
| 0 | 5 | -5494.99348657106 | 0 | 6 | 27386.1918081797 | 0 | 7 | -75861.4334859187 |
| 1 | 5 | -48814.0360404613 | 1 | 6 | 210387.578621541 | 1 | 7 | -529386.428965916 |
| 2 | 5 | 283940.662885404 | 2 | 6 | -1261022.76787976 | 2 | 7 | 3245873.44871437 |
| 3 | 5 | -573728.968470894 | 3 | 6 | 2555763.80515297 | 3 | 7 | -6616167.17139263 |
| 4 | 5 | 496377.262929330 | 4 | 6 | -2204123.17465255 | 4 | 7 | 5709449.19416504 |
| 5 | 5 | -156654.734823045 | 5 | 6 | 692217.214417601 | 5 | 7 | -1791097.75814672 |
| 0 | 8 | 119842.7335425191 | 0 | 9 | -102512.0022381539 | 0 | 10 | 37289.02112395763 |
| 1 | 8 | 772629.7133831963 | 1 | 9 | -602015.7939424901 | 1 | 10 | 191935.0886259170 |
| 2 | 8 | -4822352.035766482 | 2 | 9 | 3827647.162865941 | 2 | 10 | -1252416.581031599 |
| 3 | 8 | 9899400.748726800 | 3 | 9 | -7926981.606755933 | 3 | 10 | 2624017.867952236 |
| 4 | 8 | -8566713.640416473 | 4 | 9 | 6892074.424087163 | 4 | 10 | -2297051.762950559 |
| 5 | 8 | 2690518.369643806 | 5 | 9 | -2171115.032010596 | 5 | 10 | 727184.6991137798 |

**Table S2:** Parametrization of $c_3^{(q_1\,q_2\,q_3)} = \sum_{k=0}^{5} a_3^{(k\,q_1\,q_2\,q_3)} \left(\frac{T_e}{31577\,\mathrm{K}}\right)^k$ for the three-body term $\Phi_3$, see Eq. (S3).

| $k$ | $q_1$ | $q_2$ | $q_3$ | $a_3^{(k\,q_1\,q_2\,q_3)}$ | $k$ | $q_1$ | $q_2$ | $q_3$ | $a_3^{(k\,q_1\,q_2\,q_3)}$ |
|---|---|---|---|---|---|---|---|---|---|
| 0 | 2 | 2 | 0 | -0.484742122936188 | 0 | 2 | 3 | 0 | 10.9087150193338 |
| 1 | 2 | 2 | 0 | -9.06449732747187 | 1 | 2 | 3 | 0 | 32.6476593724955 |
| 2 | 2 | 2 | 0 | 41.9525344564407 | 2 | 2 | 3 | 0 | -234.821794328009 |
| 3 | 2 | 2 | 0 | -73.0549723173192 | 3 | 2 | 3 | 0 | 445.128565939339 |
| 4 | 2 | 2 | 0 | 62.1731314312558 | 4 | 2 | 3 | 0 | -384.590065348177 |
| 5 | 2 | 2 | 0 | -20.9735149728352 | 5 | 2 | 3 | 0 | 128.088250726806 |
| 0 | 3 | 3 | 0 | -26.51412956990250 | 0 | 2 | 2 | 1 | 22.1886312645380 |
| 1 | 3 | 3 | 0 | -41.48716191137632 | 1 | 2 | 2 | 1 | -35.1166767655775 |
| 2 | 3 | 3 | 0 | 401.5597155688950 | 2 | 2 | 2 | 1 | -105.001706438450 |
| 3 | 3 | 3 | 0 | -772.0788345667706 | 3 | 2 | 2 | 1 | 325.429922575188 |
| 4 | 3 | 3 | 0 | 646.0081532301424 | 4 | 2 | 2 | 1 | -302.151293271689 |
| 5 | 3 | 3 | 0 | -204.8877088427139 | 5 | 2 | 2 | 1 | 96.1147759289952 |
| 0 | 2 | 3 | 1 | -120.252372821342 | 0 | 3 | 3 | 1 | 183.1217840071796 |
| 1 | 2 | 3 | 1 | 159.047356694074 | 1 | 3 | 3 | 1 | -288.3551841733145 |
| 2 | 2 | 3 | 1 | 749.046048760271 | 2 | 3 | 3 | 1 | -936.8320057795876 |
| 3 | 2 | 3 | 1 | -2216.09205938898 | 3 | 3 | 3 | 1 | 3190.569713601079 |
| 4 | 2 | 3 | 1 | 2126.62367753068 | 4 | 3 | 3 | 1 | -3291.696853590043 |
| 5 | 2 | 3 | 1 | -707.455756431839 | 5 | 3 | 3 | 1 | 1159.300998652859 |

*continuation on next page ...*

*continuation from last page*

| $k$ | $q_1$ | $q_2$ | $q_3$ | $a_3^{(k\,q_1\,q_2\,q_3)}$ | $k$ | $q_1$ | $q_2$ | $q_3$ | $a_3^{(k\,q_1\,q_2\,q_3)}$ |
|---|---|---|---|---|---|---|---|---|---|
| 0 | 2 | 2 | 2 | -19.4315027093624 | 0 | 2 | 3 | 2 | 96.3144087590581 |
| 1 | 2 | 2 | 2 | 42.1788604704338 | 1 | 2 | 3 | 2 | -173.588114464854 |
| 2 | 2 | 2 | 2 | 9.67634296126227 | 2 | 2 | 3 | 2 | -157.818542202707 |
| 3 | 2 | 2 | 2 | -141.700074704502 | 3 | 2 | 3 | 2 | 751.291373937404 |
| 4 | 2 | 2 | 2 | 157.523635751903 | 4 | 2 | 3 | 2 | -702.941624093910 |
| 5 | 2 | 2 | 2 | -54.5952459846017 | 5 | 2 | 3 | 2 | 212.581414043121 |
| 0 | 3 | 3 | 2 | -54.77774286211852 | 0 | 2 | 2 | 3 | -65.4726886857960 |
| 1 | 3 | 3 | 2 | -33.08913487085887 | 1 | 2 | 2 | 3 | 102.053920198204 |
| 2 | 3 | 3 | 2 | 882.6375062820463 | 2 | 2 | 2 | 3 | 425.612227408026 |
| 3 | 3 | 3 | 2 | -1948.237600009282 | 3 | 2 | 2 | 3 | -1403.05615543312 |
| 4 | 3 | 3 | 2 | 1568.964792883849 | 4 | 2 | 2 | 3 | 1437.50728878185 |
| 5 | 3 | 3 | 2 | -439.1908951980764 | 5 | 2 | 2 | 3 | -504.993626721485 |
| 0 | 2 | 3 | 3 | 336.447897505456 | 0 | 3 | 3 | 3 | -420.786323757512 |
| 1 | 2 | 3 | 3 | -507.178567927645 | 1 | 3 | 3 | 3 | 602.981897592014 |
| 2 | 2 | 3 | 3 | -2093.07884553079 | 2 | 3 | 3 | 3 | 2804.76991700882 |
| 3 | 2 | 3 | 3 | 6834.03239451122 | 3 | 3 | 3 | 3 | -8941.73384478093 |
| 4 | 2 | 3 | 3 | -6988.05320202182 | 4 | 3 | 3 | 3 | 9095.82514910275 |
| 5 | 2 | 3 | 3 | 2453.90944239108 | 5 | 3 | 3 | 3 | -3187.19934480896 |

**Table S3:** Parametrization of $c_\rho^{(q_1\,q_2)} = \sum_{k=0}^{5} a_\rho^{(k\,q_1\,q_2)} \left(\frac{T_\mathrm{e}}{31577\,\mathrm{K}}\right)^k$ for the embedding function $\Phi_\rho$, see Eq. (S5).

| $k$ | $q_1$ | $q_2$ | $a_\rho^{(k\,q_1\,q_2)}$ | $k$ | $q_1$ | $q_2$ | $a_\rho^{(k\,q_1\,q_2)}$ |
|---|---|---|---|---|---|---|---|
| 0 | 2 | 1 | -14.1226298367901 | 0 | 2 | 2 | 15.1973595898918 |
| 1 | 2 | 1 | 42.8178754251152 | 1 | 2 | 2 | -76.2426696199033 |
| 2 | 2 | 1 | -46.9725273143709 | 2 | 2 | 2 | 180.466580679766 |
| 3 | 2 | 1 | -7.49328100982082 | 3 | 2 | 2 | -227.822610054901 |
| 4 | 2 | 1 | 50.9341743266501 | 4 | 2 | 2 | 143.162975148651 |
| 5 | 2 | 1 | -26.0690457870547 | 5 | 2 | 2 | -34.7706099024473 |

**Table S4:** Parametrization of the Helmholtz free energy of an isolated atom $\Phi_0(T_\mathrm{e})$, see Eq. (S10).

| $k$ | $a_0^{(k)}$ | $k$ | $a_0^{(k)}$ | $k$ | $a_0^{(k)}$ |
|---|---|---|---|---|---|
| 0 | -102.905307363449 | 1 | -10.3921123486934 | 4 | -1.06389593948069 |
| 5 | 12.4244554652269 | 6 | -183.607940058980 | 7 | 816.889082583121 |
| 8 | -1946.46133504029 | 9 | 2899.84763931852 | 10 | -2817.24323376719 |
| 11 | 1750.31164692968 | 12 | -635.201199559016 | 13 | 102.801048351004 |

# 3 Fortran implementation of the interatomic potential

The provided file `calc_Si_Phi_of_Te_module.f90` contains a Fortran subroutine, which calculates the forces and the Helmholtz free structural energy of a system of atoms from our interatomic potential at a given electronic temperature $T_\mathrm{e}$. The subroutine reads the input variables `NumAt, MaxNumNeib, PBC, BoxLength, coord, Te` and sets the output variables `force, energy, info` without using any global variables. In the following, we list the meaning of selected internal program variables:

`Nr2` $\triangleq N_2^{(r)}$, `Nr3` $\triangleq N_3^{(r)}$, `Nt3` $\triangleq N_3^{(\theta)}$, `Nrhorho` $\triangleq N_\rho^{(\rho)}$, `Nrrho` $\triangleq N_\rho^{(r)}$,

`Rc2` $\triangleq r_2^{(\mathrm{c})}$, `Rc3` $\triangleq r_3^{(\mathrm{c})}$, `Rcrho` $\triangleq r_\rho^{(\mathrm{c})}$, `mIRc2` $\triangleq -1/r_2^{(\mathrm{c})}$, `mIRc3` $\triangleq -1/r_3^{(\mathrm{c})}$,

`mIRcrho` $\triangleq -1/r_\rho^{(\mathrm{c})}$, `maxRc` $\triangleq \max\left(r_2^{(\mathrm{c})}, r_3^{(\mathrm{c})}, r_\rho^{(\mathrm{c})}\right)$, `maxRc2` $\triangleq \max\left(r_2^{(\mathrm{c})}, r_3^{(\mathrm{c})}, r_\rho^{(\mathrm{c})}\right)^2$,

`rhoi(q2)` $\triangleq \rho_i^{(q_2)}$, `arhoipower(q1,q2)` $\triangleq \left(\frac{\rho_i^{(q_2)}}{1+\rho_i^{(q_2)}}\right)^{q_1}$, `cosijk` $\triangleq \cos(\theta_{ijk})$,

`cosijkpower(q3)` $\triangleq \cos(\theta_{ijk})^{q_3}$, `rij` $\triangleq r_{ij}$, `rik` $\triangleq r_{ik}$, `Irij` $\triangleq 1/r_{ij}$, `Irik` $\triangleq 1/r_{ik}$.

The unit of `Te` is K, of `energy` is eV, of `force` is eV/Å, of `coord` and `BoxLength` is Å.
